# Supplementary material for: Graph Pruning for Enumeration of Minimal Unsatisfiable Subsets
Source: arXiv:2402.15524 source file (2024-02-19)
Supplement: Supplementary file 1 [file appendix.tex]

\clearpage
\section*{Appendix}

\subsection*{Problem generation}
In this section we provide details on the problem generation parameters for our experiments.
\begin{table}[h]
    \centering
    \begin{tabular}{|c|c|c|c|}
        \hline
        \textbf{Problem}    & \textbf{Pruning \%}                     \\
        \hline
        Random Formulas            &    32.22\% $\pm$ 0.83\%       \\
        \hline
        Logistics Planning              & 36.27\% $\pm$ 1.56\%          \\
        \hline
        Graph Coloring(4-7)     & 30.18\% $\pm$ 1.00\% \\
        \hline
    \end{tabular}
    \caption{Average percentage of the original formula pruned by GRAPE-MUST. }
    \label{tab:reductions}
\end{table}
\paragraph{Random Problems} We use the same generation procedure as \cite{selsam2018learning}. As mentioned in the main text, we generate formulas with 30-100 variables for our first experiment and larger formulas for testing Extrapolation. In our problem generation we set the parameter of the geometric distribution to 0.3. This has the effect of generating formulas with slightly more literals per clause than in \cite{selsam2018learning}. We find that this correlates with larger MUSes, which increases the difficulty of the search in our problem.

\begin{table}[h]
    \centering
    \begin{tabular}{|c|c|}
        \hline
        \textbf{\# Variables}    & \textbf{Pruning \%}         \\            
        \hline
        100           &    30.22\% $\pm$ 0.83\%       \\
        \hline
        150             & 29.16\% $\pm$ 1.14\%          \\
        \hline
        200     & 27.68\% $\pm$ 1.26\% \\
        \hline
        250     & 24.28\% $\pm$ 1.45\% \\
        \hline
        300     & 23.48\% $\pm$ 1.48\%\\
        \hline
    \end{tabular}
    \caption{Average percentage of the original formula pruned by GRAPE-MUST. }
    \label{tab:extrap_reductions}
\end{table}
\begin{table*}[h]
    \footnotesize
    \begin{tabular}{|c|c|c|c|c|c|}
        \hline
        \textbf{Solver}    & \textbf{100 vars.}          & \textbf{150 vars.}          & \textbf{200 vars.}         & \textbf{250 vars.}         & \textbf{300 vars.}        \\
        \hline
        MARCO              & 1145.92$\pm$ 36.0           & 348.56$\pm$ 17.84           & 103.0$\pm$ 8.13            & 55.6$\pm$ 7.52             & 19.33$\pm$ 3.31           \\
        GRAPE-MUST + MARCO & \textbf{1157.69$\pm$ 34.03} & \textbf{357.43$\pm$ 17.98}  & \textbf{108.21$\pm$ 8.47}  & \textbf{60.31$\pm$ 8.7}    & \textbf{20.25$\pm$ 3.31}  \\
        \hline
        Remus              & 5188.03$\pm$ 149.6          & 1493.73$\pm$ 77.36          & 404.66$\pm$ 35.97          & 156.41$\pm$ 19.74          & 63.29$\pm$ 14.78          \\
        GRAPE-MUST + REMUS & \textbf{1157.69$\pm$ 34.03} & \textbf{2216.71$\pm$ 91.92} & \textbf{630.75$\pm$ 50.52} & \textbf{220.49$\pm$ 25.72} & \textbf{66.38$\pm$ 11.69} \\
        \hline
        Tome               & 723.29$\pm$ 23.32           & 218.99$\pm$ 9.81            & 68.02$\pm$ 4.56            & 30.31$\pm$ 3.03            & 11.13$\pm$ 1.75           \\
        GRAPE-MUST + TOME  & \textbf{848.8$\pm$ 27.96}   & \textbf{244.87$\pm$ 11.11}  & \textbf{76.67$\pm$ 5.03}   & \textbf{35.56$\pm$ 3.42}   & \textbf{12.86$\pm$ 2.02}  \\
        \hline
    \end{tabular}
    \caption{Enumeration results from the extrapolation experiment.}
    \label{tab:extrap_enumeration}
\end{table*}

\paragraph{Graph coloring}
The generation parameters are summarized in the text. We follow a standard SAT encoding for graph coloring problems: Each node is associated with at-least-1 and at-most-one constraints for the colors. Each edge is represented by K clauses for K colors, forbidding adjacent nodes to share that color. To plot pruned graph coloring formulas as graphs, the pruned formula is further processed for visualization using pure literal elimination to remove clauses that are trivially satisfiable.

\paragraph{Logistics planning}
The domain file for the logistics planning problem is available along-side our code. Unfortunately we could not obtain permission to distribute the planner with our code in time, however it is available online at https://research.ics.aalto.fi/software/sat/madagascar/ freely for academic purposes. We generate trajectories of up to 5 steps with 5 to 10 packages, 1 airplane, 2 airports, 2 cities, 2 locations, and 2 trucks, which are all matched randomly with each other in the initial and goal states. We use the following command line options to generate the problems: \verb|-P 0 -1 -O -S 1 -F <steps>-1 -T <steps>|

\begin{table*}[!ht]
    \centering
    \begin{tabular}{|c|c|c|c|}
        \hline
        \textbf{Solver (30 mins.)} & \textbf{Random Problems} & \textbf{Logistics Planning} & \textbf{Graph Coloring}  \\ \hline
        Marco                      & $96220 \pm 7129$         & $172933.72 \pm 16285.18$    & $128638.94 \pm 23702.68$ \\
        GRAPE-MUST + Marco         & $97254 \pm 6822$         & $177356.60 \pm 16373.36$    & $176703.96 \pm 31061.28$ \\ \hline
        Remus                      & $484033 \pm 25554$       & $82774.54 \pm 5690.20$      & $8965.48 \pm 1121.03$    \\
        GRAPE-MUST + Remus         & $504056 \pm 28010$       & $87825.64 \pm 6239.49$      & $15525.12 \pm 3201.24$   \\ \hline
        Tome                       & $73644 \pm 3318$         & $24403.12 \pm 2843.69$      & $72476.06 \pm 16174.54$  \\
        GRAPE-MUST + Tome          & $73442 \pm 3719$         & $25903.40 \pm 2842.90$      & $54981.82 \pm 12340.48$  \\ \hline
    \end{tabular}
    \caption{Average number of MUSes found by each solver in 30 minutes.}
    \label{tab:longer_timeout}
\end{table*}
\subsection*{Longer timeout experiment}

In this section we show the results from a smaller scale experiment with a longer timeout. We use the same problem generation parameters as in the main text, but we use a 30 minute timeout instead. The results are shown in Table \ref{tab:longer_timeout}.

In random problems, pruned formulas still result in more MUSes found by Marco and Remus, but the difference is proportionally smaller than in shorter time limits. In fact, Tome finds almost the same number of MUSes in both formulas on average. Similarly, in logistics planning problems pruning still benefits all solvers but the effect is not as strong in the longer time limit. In graph coloring problems, pruning still offers significant benefit to Marco and Remus, while it seems to disrupt Tome's search strategy consistent with our experiment in section 5.1.

Overall, while even in longer time limits solvers with different search strategies interact with GRAPE-MUST differently, the combination GRAPE-MUST+REMUS consistently outperforms other methods in our experiments. Furthermore, the results from random and logistics planning problems indicate that given enough time, the speed-up due to pruning may diminish. However, as demonstrated in section 5.3, in realistic problems with a standard time limit of 2 hours GRAPE-MUST offers significant benefit to MUS enumeration in most cases.

\subsection*{Extrapolation experiment additional tables}

Here we show the reduction and enumeration results for the extrapolation experiment in additional detail.

Table \ref{tab:extrap_reductions} Shows that formula pruning performance is fairly consistent even in larger problem sizes, with the pruning percentage decreasing by about 7 percentage points when the problem, size is tripled. This indicates that the pruning method that the model has learned is able to generalize to larger problems and can therefore be used to accelerate MUS enumeration on larger problems.

Table \ref{tab:extrap_enumeration} Shows the detailed MUS enumeration performance before and after pruning for the extrapolation experiment. As discussed in the main text, GRAPE-MUST is able to accelerate MUS enumeration especially for REMUS in larger problems. Interestingly, around 200 variables, the improvement of REMUS is even higher than previous results, indicating a sweet-spot between extrapolation ability and problem size.

\subsection*{Pruning statistics}

Table \ref{tab:reductions} shows the average percentage of clauses pruned by our model. We can see that GRAPE-MUST actually prunes a significant fraction of the clauses in the original formulas. We have also tried a random pruning method that randomly removes the same fraction of clauses, and the resulting formulas are mostly satisfiable. This provides further evidence that our pruning model can effectively identify non-critical constraints.

\subsection*{Comparison with naive pruning}
We devise the following two naive strategies and apply them to the collection of hard problems from the 2011 SAT competition MUS enumeration benchmark used in the main text. To make the comparison with our method fair, both strategies involve O(1) SAT calls with respect to the problem size. We use the following two strategies to rank clauses:
\begin{itemize}
    \item  Clause-length based: Given a problem $S = (U,C)$ Let $l_{max}= \max_{c \in C} |c|$ and $l_{min}= \min_{c \in C} |c|$. Then, taking K=100 equally sized integer steps between $l_{max}$ and $l_{min}$ search for the smallest clause length $l^*$ such that $C' = {c \in C, |c|\leq l^*}$ and $S' = (C',U')$ is unsatisfiable. Return  $S'$.
    \item Variable frequency based: Compute the frequency in which each variable (and its negation) appear in the clauses of S. Then, each clause is scored by the negative average frequency of the variables (and their negations) in it. As a result, clauses with variables appearing in few other clauses receive higher scores. Then, prune the formula as in the previous strategy, only using clause scores instead of length to decide pruning. This replaces scores produced by our GNN.
\end{itemize}

The first strategy produces on average formulas $0.08\%$ smaller than the original formulas, with most problems not being successfully pruned. Most problems failed to be pruned after a single SAT call, taking little time from MUS enumeration. As a result, 55 of the benchmark problems have the same number of MUSes enumerated between the two methods. The clause-length strategy improves enumeration in 5 problems and reduces the number of MUSes found in 3 problems.  Interestingly, in one of the problems where the first strategy succeeds, REMUS finds 1 MUS, GRAPE-MUST + REMUS finds 13 and  Strategy 1 + REMUS finds 134. This may suggest that for some problems, naive heuristics like clause-length may be viable strategies, however it is not clear how to decide in which problems to use it and it does not generalize well. Since GRAPE-MUST is a learning model trained on difficult random problems, its learned heuristic is much more widely applicable, even if better problem-specific heuristics may exist. The second strategy prunes no formulas successfully, and so we do not run MUS enumeration.
\newpage
\section*{Checklist}

% %%% BEGIN INSTRUCTIONS %%%
%The checklist follows the references. For each question, choose your answer from the three possible options: Yes, No, Not Applicable.  You are encouraged to include a justification to your answer, either by referencing the appropriate section of your paper or providing a brief inline description (1-2 sentences).
%Please do not modify the questions.  Note that the Checklist section does not count towards the page limit. Not including the checklist in the first submission won't result in desk rejection, although in such case we will ask you to upload it during the author response period and include it in camera ready (if accepted).

%\textbf{In your paper, please delete this instructions block and only keep the Checklist section heading above along with the questions/answers below.}
% %%% END INSTRUCTIONS %%%

\begin{enumerate}

    \item For all models and algorithms presented, check if you include:
          \begin{enumerate}
              \item A clear description of the mathematical setting, assumptions, algorithm, and/or model. [Yes]
              \item An analysis of the properties and complexity (time, space, sample size) of any algorithm. [Yes]
              \item (Optional) Anonymized source code, with specification of all dependencies, including external libraries. [Yes]
          \end{enumerate}

    \item For any theoretical claim, check if you include:
          \begin{enumerate}
              \item Statements of the full set of assumptions of all theoretical results. [Not Applicable]
              \item Complete proofs of all theoretical results. [Not Applicable]
              \item Clear explanations of any assumptions. [Not Applicable]
          \end{enumerate}

    \item For all figures and tables that present empirical results, check if you include:
          \begin{enumerate}
              \item The code, data, and instructions needed to reproduce the main experimental results (either in the supplemental material or as a URL). [Yes]
              \item All the training details (e.g., data splits, hyperparameters, how they were chosen). [Yes]
              \item A clear definition of the specific measure or statistics and error bars (e.g., with respect to the random seed after running experiments multiple times). [Yes]
              \item A description of the computing infrastructure used. (e.g., type of GPUs, internal cluster, or cloud provider). [Yes]
          \end{enumerate}

    \item If you are using existing assets (e.g., code, data, models) or curating/releasing new assets, check if you include:
          \begin{enumerate}
              \item Citations of the creator If your work uses existing assets. [Yes]
              \item The license information of the assets, if applicable. [Yes]
              \item New assets either in the supplemental material or as a URL, if applicable. [Yes]
              \item Information about consent from data providers/curators. [Not Applicable]
              \item Discussion of sensible content if applicable, e.g., personally identifiable information or offensive content. [Not Applicable]
          \end{enumerate}

    \item If you used crowdsourcing or conducted research with human subjects, check if you include:
          \begin{enumerate}
              \item The full text of instructions given to participants and screenshots. [Not Applicable]
              \item Descriptions of potential participant risks, with links to Institutional Review Board (IRB) approvals if applicable. [Not Applicable]
              \item The estimated hourly wage paid to participants and the total amount spent on participant compensation. [Not Applicable]
          \end{enumerate}

\end{enumerate}
